# Supplementary material for: Tractable MCMC for Private Learning with Pure and Gaussian Differential Privacy
Source: arXiv:2310.14661 source file (2024-05-01)
Supplement: Supplementary file 1 [file OutPert_appendix.tex]

We restate the Algorithm~\ref{alg:outpert} in Algorithm~\ref{alg:outpert_2}. Note that in step~\ref{opt_oracle_2}, knowing the exact value of $\theta^*$ is not required. That is because $\|\Tilde{\theta}-\theta^*\|_2 \leq \frac{\tau}{n}$ is not a stopping criteria of the optimization algorithm. Instead, it is a property that $\Tilde{\theta}$ would fulfill under the stopping criteria the additional assumption on $\cL$. 
\begin{algorithm}
\caption{Approximate Output Perturbation}
\label{alg:outpert_2}
    \begin{algorithmic}[1]
        \State \textbf{Input:} individual losses $\{\ell_i\}_{i=1}^n$ satisfying $G$-Lipschitz continuity and $\beta$-smoothness; average local strong convexity parameter $\alpha$; $\tau$
        \State Denote $\cL(\theta) := \sum_{i=1}^n \ell_{i}(\theta)$.
        \State Denote $\theta^*:= \argmin_{\theta} \cL(\theta)$
        \State Find $\Tilde{\theta}$ that satisfies $\|\Tilde{\theta}-\theta^*\|_2 \leq \frac{\tau}{n}$. \label{opt_oracle_2}
        \State Set $\Tilde{\Delta} := \frac{2\tau}{n} + \frac{2G}{\alpha n}$.
        \State Output $\theta_0 = \Tilde{\theta} + \boldsymbol{Z}$, where $\boldsymbol{Z}_i \sim \text{Lap}(\frac{\sqrt{d}\Tilde{\Delta}}{\varepsilon})$ for $\varepsilon$-pure DP ($\boldsymbol{Z}_i \sim \cN(0, \frac{\Tilde{\Delta}^2}{\mu^2})$ for $\mu$-GDP).
    \end{algorithmic}
\end{algorithm}

An instantiation of the optimization oracle is the Newton Descent, which converges linearly under the assumption of $c$-stable Hessian by the Theorem 2 of \cite{karimireddy2018global}. We restate the Algorithm~\ref{alg:ND_oracle} in Algorithm~\ref{alg:ND_oracle_2} and show that Step~\ref{opt_oracle_2} can be satisfied by Algorithm~\ref{alg:ND_oracle_2}.

\begin{algorithm}
[h!]
\caption{Newton Descent Oracle} \label{alg:ND_oracle_2}
\begin{algorithmic}
    \State{Input: initial point $\Tilde{\theta}_0$, domain $\cQ$, $\cL(\tilde{\theta})$ that satisfies $c$-stable Hessian, individual losses $\{\ell_i\}_{i=1}^n$ satisfying $G$-Lipschitz continuity and $\beta$-smoothness, step size $\sigma$, number of iterations $T$ }
    \For{$t = 0,1,2, \ldots , T-1$}
    \State $\tilde{\theta}_{t+1}\leftarrow \tilde{\theta}_t-\frac{1}{\sigma}[\nabla^2 \cL (\tilde{\theta}_t)]^\dagger \nabla \cL (\tilde{\theta}_t)$
    \EndFor
    \State{Return:  $\tilde{\theta} =\tilde{\theta}_T$}
\end{algorithmic}
\end{algorithm}

We first provide the definition of $c$-stable Hessian \citep{karimireddy2018global}.
\begin{assumption}[c-stable Hessian, \citep{karimireddy2018global}]\label{def:c_stable_Hessian}
For any $u,v \in \mathcal{Q}$ and $u\neq v$, we assume that $\| v-u\|_{\nabla^2 \cL(u)}>0$ and that there exists a constant $c \geq 1$ such that 
\[
c = \max_{u,v \in \cQ} \frac{\| v-u\|^2_{\nabla^2 \cL(v)}}{\| v-u\|^2_{\nabla^2 \cL(u)}} = \max_{u,v \in \cQ} \frac{(v-u)^T \nabla^2 \cL(v) (v-u)}{(v-u)^T \nabla^2 \cL(u) (v-u)}
\]
\end{assumption}

\begin{lemma}[Lemma 2 of \cite{karimireddy2018global}]
\label{lem:c_stable_Hessian}
    Given Assumption~\ref{def:c_stable_Hessian}, for any $u,v \in \cQ$, we have 
    \[
    \cL(u) \geq \cL(v)+ \langle \nabla \cL(v), u-v \rangle + \tfrac{1}{2c}\| u-v\|^2_{\nabla^2 \cL(v)}.
    \]
\end{lemma}

    We use the above Lemma~\ref{lem:c_stable_Hessian} to show that Step~\ref{opt_oracle_2} can be satisfied by Algorithm~\ref{alg:ND_oracle_2}. Taking $v=\theta^*$ and $u=\tilde{\theta}$, we have that
    \[
    2c\lrp{\cL(\tilde{\theta}) -\cL(\theta^*)}\geq\| \theta^*-\tilde{\theta}\|^2_{\nabla^2 \cL(\theta^*)} \geq \alpha n\| \theta^*-\tilde{\theta}\|^2.        
    \]
    Therefore $\| \theta^*-\tilde{\theta}\| \leq \sqrt{\frac{2c}{\alpha n}}\sqrt{\lrp{\cL(\tilde{\theta}) -\cL(\theta^*)}}$.

 The following lemma demonstrates that Algorithm~\ref{alg:ND_oracle_2} converges linearly. 
 
\begin{lemma}[Theorem 2 of \cite{karimireddy2018global}]
    Given Assumption \ref{def:c_stable_Hessian}, for any iteration $T>0$ of Algorithm \ref{alg:ND_oracle_2} with $\sigma \geq c$,
\[
\cL(\tilde{\theta}_T)-\cL(\theta^*) \leq (1-\frac{1}{c\sigma })^T[\cL(\tilde{\theta}_0)-\cL(\theta^*)].
\]
\end{lemma}

Therefore with $T=\frac{\ln{n}+2\ln\lrp{1/\tau}+\ln(2c/\alpha)+\ln\lrp{\cL(\tilde{\theta}_0) -\cL(\theta^*)}}{-\ln(1-\frac{1}{c\sigma})}$  iterations, Algorithm~\ref{alg:ND_oracle_2} will converge to a $\tilde{\theta}$ that satisfy Step~\ref{opt_oracle_2} in Algorithm~\ref{alg:outpert_2}.

We provide the omitted proofs of Lemma~\ref{lem:sensitivity_minimizer} and Lemma~\ref{lem:OutPert_DP}. 

\begin{proof}[Proof of Lemma~\ref{lem:sensitivity_minimizer}]
    By $\alpha$ average local strong convexity and first-order optimality conditions
    \begin{align*}
    \cL_D(\theta^*(D'))  &\geq \cL_D(\theta^*(D)) + \langle \theta^*(D') - \theta^*(D), \nabla \cL(D)(\theta^*(D))\rangle  + \frac{\alpha n}{2}\| \theta^*(D)  - \theta^*(D') \|^2 \\
    &\geq \frac{\alpha n}{2}\| \theta^*(D)  - \theta^*(D') \|^2.
    \end{align*}
    By convexity of $\cL_{D'}$ and first order optimality condition for $\theta^*(D')$
    $$\cL_{D'}(\theta^*(D))  \geq \cL_{D'}(\theta^*(D')) + \langle \theta^*(D) - \theta^*(D'), \nabla \cL(D')(\theta^*(D'))\rangle \geq 0.$$
    Add the two inequalities we get 
    \begin{align*}
    \frac{\alpha n}{2}\| \theta^*(D)  - \theta^*(D') \|^2 &\leq \cL_D(\theta^*(D')) - \cL_{D'}(\theta^*(D')) + \cL_{D'}(\theta^*(D))  -  \cL_D(\theta^*(D)) \\
    &\leq |\ell_x(\theta^*(D')) - \ell_x(\theta^*(D))| \leq G\| \theta^*(D)  - \theta^*(D') \|.
    \end{align*}
    The proof is complete by dividing both sides by $\| \theta^*(D)  - \theta^*(D') \|$.
\end{proof}

\begin{proof}[Proof of Lemma~\ref{lem:OutPert_DP}]
    It suffices to show the sensitivity of $\Tilde{\theta}(D)$ is bounded by $\Tilde{\Delta}$.
    The sensitivity of $\Tilde{\theta}(D)$ is  bounded by 
\begin{align*}
    \max_{D \simeq D'} || \Tilde{\theta}(D) -  \Tilde{\theta}(D') ||_2 &= \max_{D \simeq D'} || \Tilde{\theta}(D) - \theta^*(D) + \theta^*(D) - \theta^*(D') + \theta^*(D')  -\Tilde{\theta}(D')||_2 \\
    &\leq  || \Tilde{\theta}(D) - \theta^*(D)||_2 + \max_{D \simeq D'} ||\theta^*(D) - \theta^*(D')||_2 + ||\theta^*(D')  -\Tilde{\theta}(D')||_2 \\
    &\leq \frac{2\tau}{n} + \frac{2G}{\alpha n}=\Tilde{\Delta}.
\end{align*}
\end{proof}
